# Supplementary material for: Modeling Token-level Uncertainty to Learn Unknown Concepts in SLU via Calibrated Dirichlet Prior RNN
Source: arXiv:2010.08101 source file (2020-10-16)
Supplement: Supplementary file 2 [file dirichlet.tex]

\section{Dirichlet Prior Illustration}\label{ap:dirichlet}

\autoref{fig:dirichlet} illustrate the high-order uncertainty measurement in Dirichlet prior network $p(\con|\vect{z}, \theta)$.
Ideally, $p(\con|\vect{z}, \theta)$ should yield sharp distribution on the corner of simplex $\mathbb{S}_k$ when the network is confident about its prediction (known-known).
For noisy input data with heavy class overlap (data uncertainty), the network should yield sharp distribution in the center of the simplex $\mathbb{S}_k$ (known-unknown).
While for out-of-distribution data, the prior network is supposed to yield flat distribution on the simplex $\mathbb{S}_k$ (unknown-unknown).
That is to say, the parameters should encapsulate the knowledge about the boundary which separates in-distribution from out-of-distribution data.
